# Supplementary material for: Model Merging in LLMs, MLLMs, and Beyond: Methods, Theories, Applications and Opportunities
Source: arXiv:2408.07666 source file (2025-12-31)
Supplement: Supplementary file 1 [file appendix.tex]

%%
%% If your work has an appendix, this is the place to put it.
\appendix

\section{Research Methods}
